# Supplementary material for: Structure, short-range order, and phase stability of the Al$_x$CrFeCoNi high-entropy alloy: Insights from a perturbative, DFT-based analysis
Source: arXiv:2404.13173 ancillary file (2024-11-28)
Supplement: Supplementary file 1 [file supplemental.pdf]

# Structure, short-range order, and phase stability of the $Al_x$CrFeCoNi high-entropy alloy: Insights from a perturbative, DFT-based analysis

Christopher D. Woodgate,[1,2,*] George A. Marchant,[1,3,†] Livia B. Pártay,[3,‡] and Julie B. Staunton[1,§]

[1]*Department of Physics, University of Warwick, Coventry, CV4 7AL, United Kingdom*
[2]*H. H. Wills Physics Laboratory, University of Bristol, Royal Fort, Bristol, BS8 1TL, United Kingdom*
[3]*Department of Chemistry, University of Warwick, Coventry, CV4 7AL, United Kingdom*

This is the supplemental material accompanying the main text. Here we provide details of lattice parameters used in our calculations, visualise the $(l, m)$-resolved electronic density of states (DoS) for selected systems, plot eigenvalues of the chemical stability matrices, and tabulate our fitted atom-atom effective pair interactions.

## I. LATTICE PARAMETERS

In Table I, we provide the fcc and bcc lattice parameters used in this study, which are consistent with their experimental values [1]. For values of $x$ where the lattice type is not observed experimentally (*e.g.* bcc, $x = 0$; fcc, $x = 2$) we perform a volume-conserving transformation from fcc to bcc structures (or vice-versa) to obtain a lattice parameter. For intermediate values of $x$ we interpolate linearly between lattice parameters in accordance with Vegard's law [2]. (The addition of Al results in a marginal expansion of the lattice.)

## II. RESOLVED DENSITY OF STATES

In Figures 1 and 2, we plot the $(l, m)$-resolved electronic DoS for the equiatomic AlCrFeCoNi system, *i.e.* $Al_x$CrFeCoNi, $x = 1$. These are obtained within the KKR formulation of DFT, using the CPA to average over disorder [3, 4]. We use the all-electron HUTSEPOT code to perform these calculations [5]. The paramagnetic state is described within the disordered local moment (DLM) picture [6–8]. Figure 1 shows results when the underlying lattice is fcc, while Figure 2 shows results when the underlying lattice is bcc. We pay particular attention to $l = 2$, *i.e.* the 3$d$ states. The $t_{2g}$ states correspond to $m = -2, -1, 1$, while the $e_g$ states correspond to $m = 0, 2$. It can be seen that there is greater splitting between the peaks in the DoS curves associated with the $e_g$ and $t_{2g}$ states when the underlying lattice is bcc.

## III. EIGENVALUES OF CHEMICAL STABILITY MATRICES

Figure 3 shows eigenvalues of the chemical stability matrix around the irreducible Brillouin zone for selected systems, constructed from the $S^{(2)}_{\alpha\alpha'}(\mathbf{k})$ data, evaluated above any disorder-order transition temperature. When the underlying lattice is fcc, a minimum at $X$ denotes an $L1_2$ ordering, while a minimum at $W$ is suggestive of a $D0_{22}$ ordering. In both cases, a minimum at $\Gamma$ is indicative of phase segregation.

## IV. EFFECTIVE PAIR INTERACTIONS

The atom-atom effective pair interactions are for the Bragg-Williams Hamiltonian [9, 10], which takes the form

$$H = \frac{1}{2} \sum_{i\alpha;j\alpha'} V_{i\alpha;j\alpha'} \xi_{i\alpha} \xi_{j\alpha'}. \tag{1}$$

* christopher.woodgate@bristol.ac.uk
† George.Marchant@warwick.ac.uk
‡ Livia.Bartok-Partay@warwick.ac.uk
§ J.B.Staunton@warwick.ac.uk

However, assuming interactions are isotropic, we can write $V^{(n)}_{\alpha\alpha'}$ to denote the interaction between species $\alpha$ and $\alpha'$ on coordination shell $n$. Then Eq. 1 takes the form

$$H = \frac{1}{2}\sum_{i}\sum_{n}\left(\sum_{j\in n(i)}\sum_{\alpha\alpha'}V^{(n)}_{\alpha\alpha'}\xi_{i\alpha}\xi_{j\alpha'}\right), \tag{2}$$

where $n(i)$ denotes the set of lattice sites which are $n$th nearest-neighbours to site $i$.

In Figures 4 and 5, we visualise the fitted effective pair interactions as a function of coordination shell number, *i.e.* radial distance, for both fcc and bcc lattices for relevant selected values of $x$. It can be seen that interactions are dominated by the first coordination shell.

For convenience, we also tabulate these effective pair interactions. Tables II, III, IV, V, and VI give our fitted effective pair interactions for the $Al_x$CrFeCoNi system on the fcc lattice for $x = 0$, 0.5, 1, 1.5, and 2, respectively. Then tables VII, VIII, IX, X, and XI give our fitted effective pair interactions for the $Al_x$CrFeCoNi system on the bcc lattice for $x = 0$, 0.5, 1, 1.5, and 2, respectively. Note that, for $x \geq 1$, the fcc structure is not expected to be stable, while for $x \leq 0.5$, the bcc structure is not expected to be stable. These results are, therefore, only provided for the purposes of comparison.


[1] W.-R. Wang, W.-L. Wang, S.-C. Wang, Y.-C. Tsai, C.-H. Lai, and J.-W. Yeh, Intermetallics **26**, 44 (2012).

[2] A. R. Denton and N. W. Ashcroft, Physical Review A **43**, 3161 (1991).

[3] H. Ebert, D. Ködderitzsch, and J. Minár, Reports on Progress in Physics **74**, 096501 (2011).

[4] J. S. Faulkner, G. M. Stocks, and Y. Wang, *Multiple Scattering Theory: Electronic Structure of Solids*, 1st ed. (IOP Publishing, Bristol, UK, 2018).

[5] M. Hoffmann, A. Ernst, W. Hergert, V. N. Antonov, W. A. Adeagbo, R. M. Geilhufe, and H. Ben Hamed, Physica Status Solidi (b) **257**, 1900671 (2020).

[6] A. J. Pindor, J. Staunton, G. M. Stocks, and H. Winter, Journal of Physics F: Metal Physics **13**, 979 (1983).

[7] J. Staunton, B. Gyorffy, A. Pindor, G. Stocks, and H. Winter, Journal of Magnetism and Magnetic Materials **45**, 15 (1984).

[8] B. L. Gyorffy, A. J. Pindor, J. Staunton, G. M. Stocks, and H. Winter, Journal of Physics F: Metal Physics **15**, 1337 (1985).

[9] W. L. Bragg and E. J. Williams, Proceedings of the Royal Society of London. Series A, Containing Papers of a Mathematical and Physical Character **145**, 699 (1934).

[10] W. L. Bragg and E. J. Williams, Proceedings of the Royal Society of London. Series A - Mathematical and Physical Sciences **151**, 540 (1935).

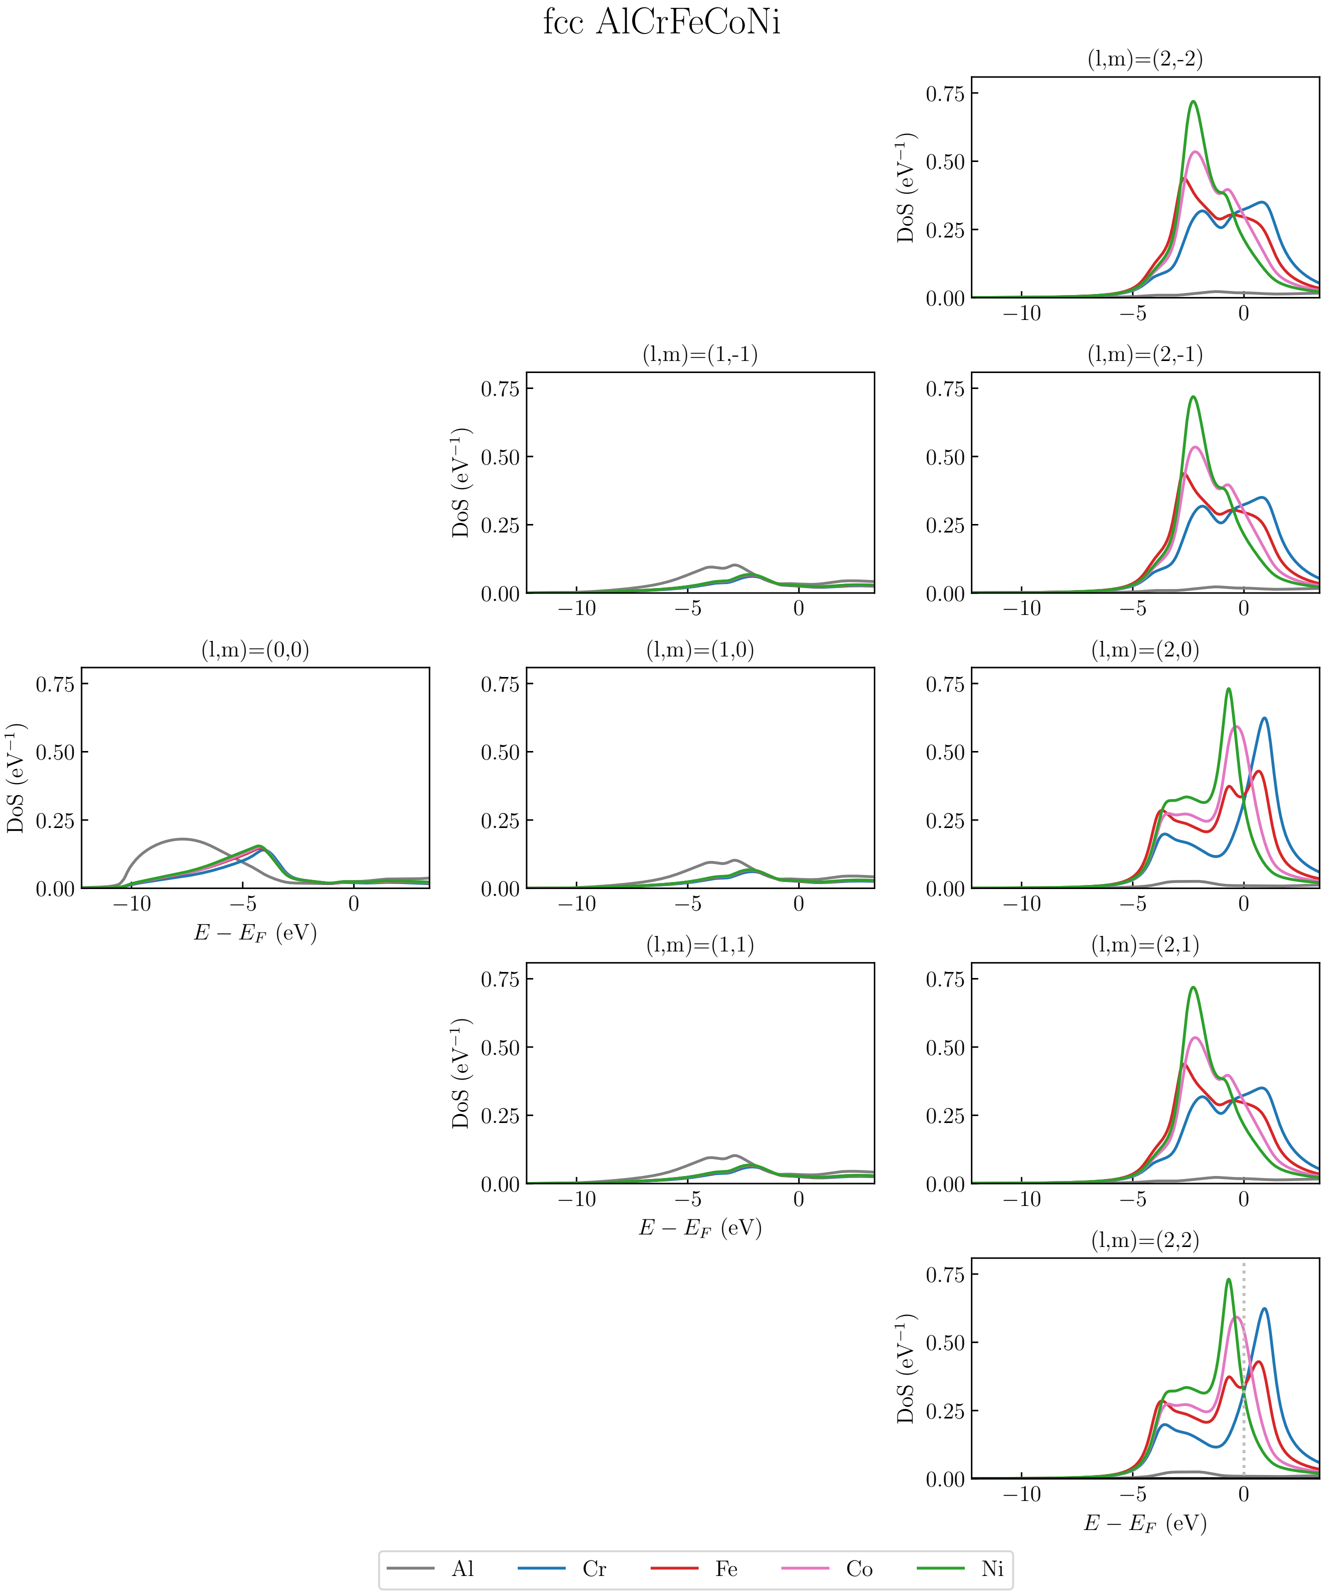


FIG. 1. $(l, m)$- and species-resolved density of states for equiatomic AlCrFeCoNi modelled on the fcc lattice.

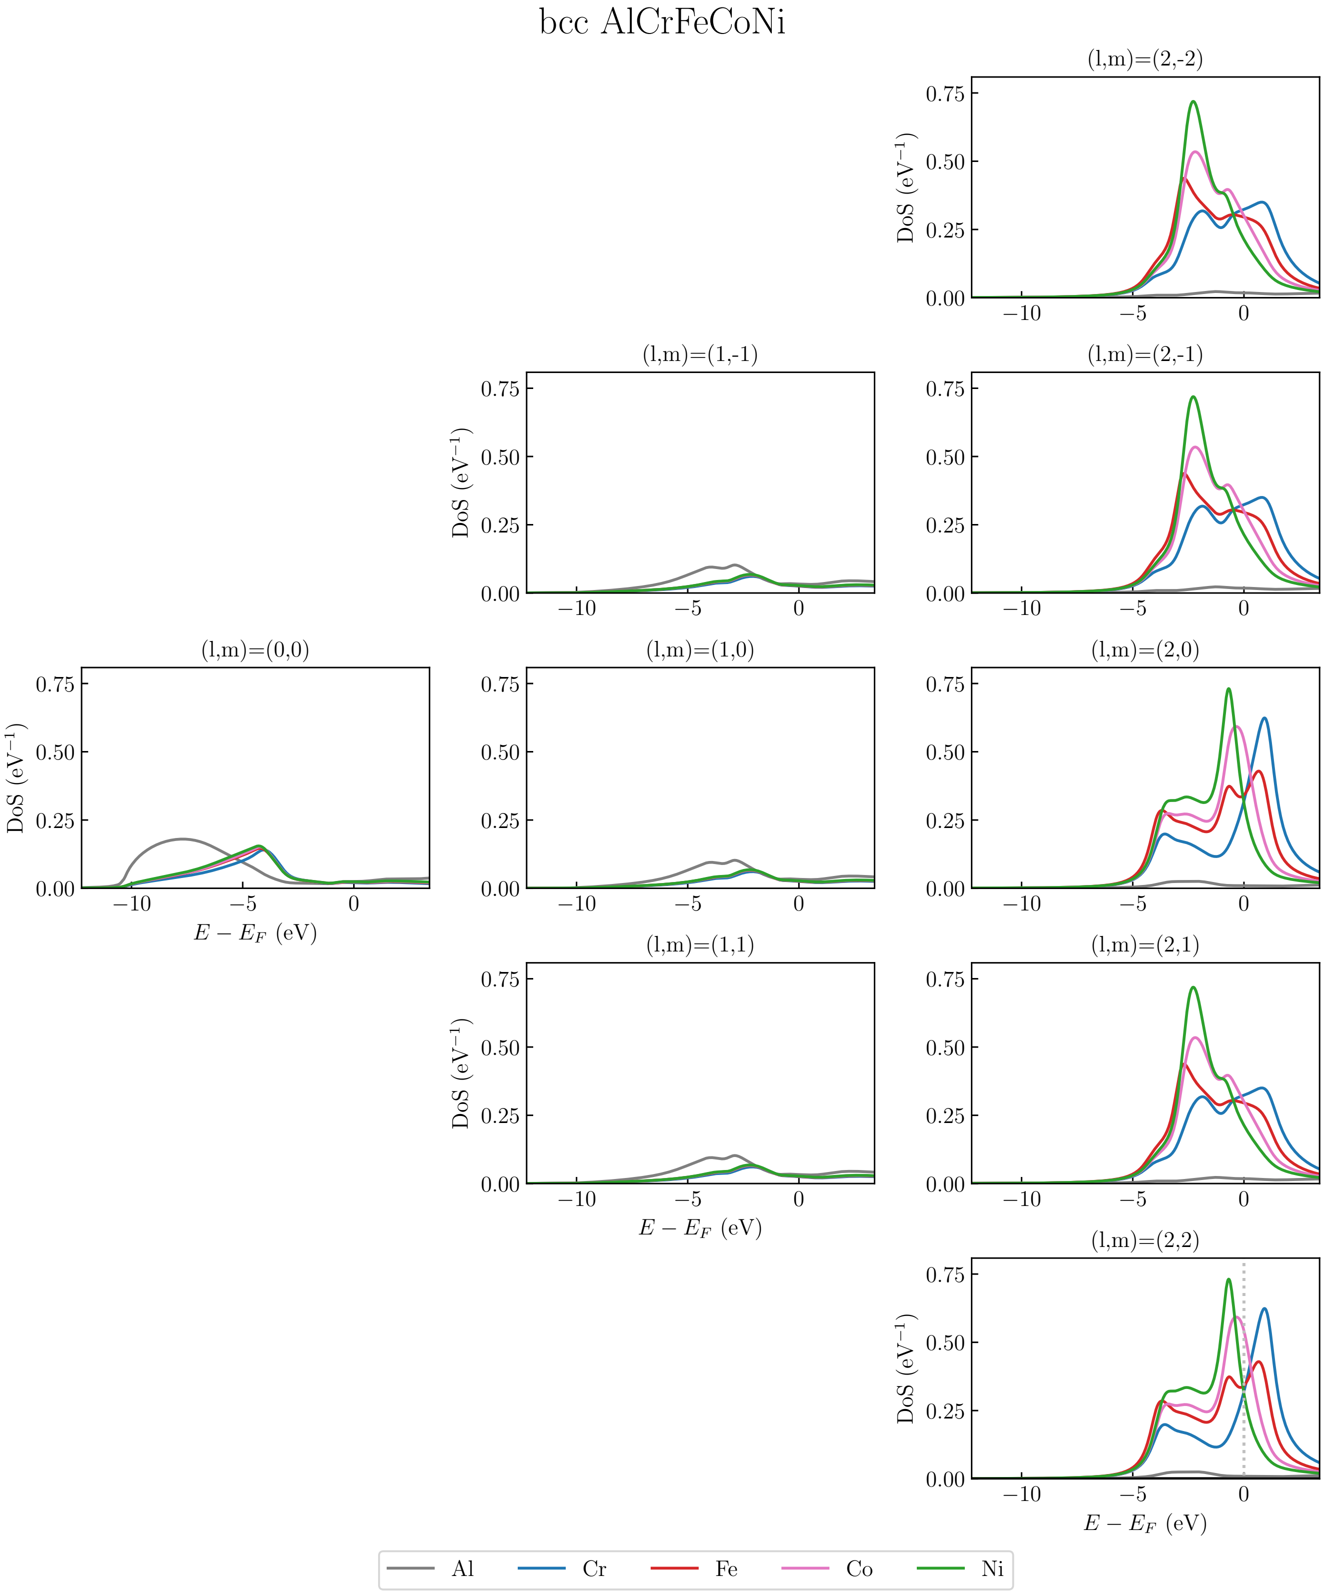


FIG. 2. $(l, m)$- and species-resolved density of states for equiatomic AlCrFeCoNi modelled on the bcc lattice.

| Al concentration, $x$ | $a_{\mathrm{fcc}}$ (Å) | $a_{\mathrm{bcc}}$ (Å) |
|---|---|---|
| 0 | 3.570 | 2.834 |
| 0.5 | 3.590 | 2.849 |
| 1 | 3.605 | 2.862 |
| 1.5 | 3.618 | 2.872 |
| 2 | 3.629 | 2.880 |

TABLE I. Lattice parameters used in this study.

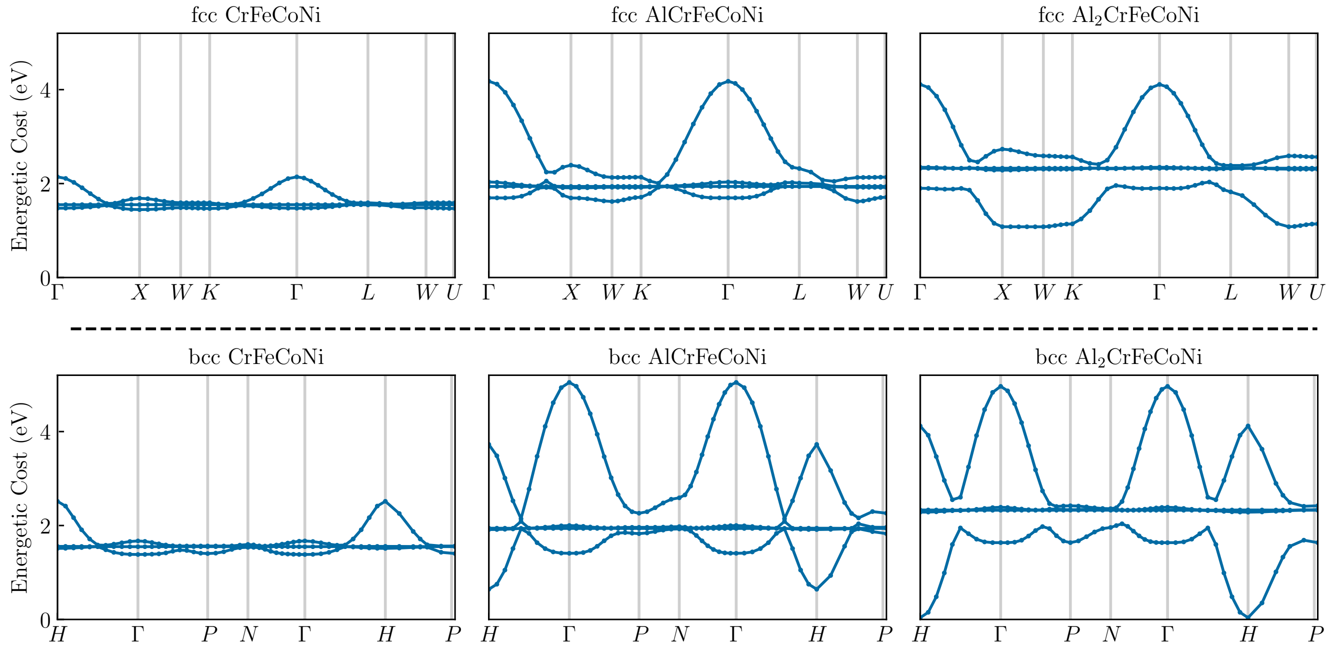


FIG. 3. Eigenvalues of the chemical stability matrix around the irreducible Brillouin zone (IBZ) for the Al$_x$CrFeCoNi system for a range of values of $x$ on both the fcc (top row) and bcc (bottom row) lattices. When the underlying lattice is bcc, a minimum at $H$ denotes a B2 ordering. When the undelying lattice is fcc, a minimum at $X$ denotes an L1$_2$ ordering, while a minimum at $W$ is suggestive of a D0$_{22}$ ordering. In both cases, a minimum at Γ is indicative of phase segregation.

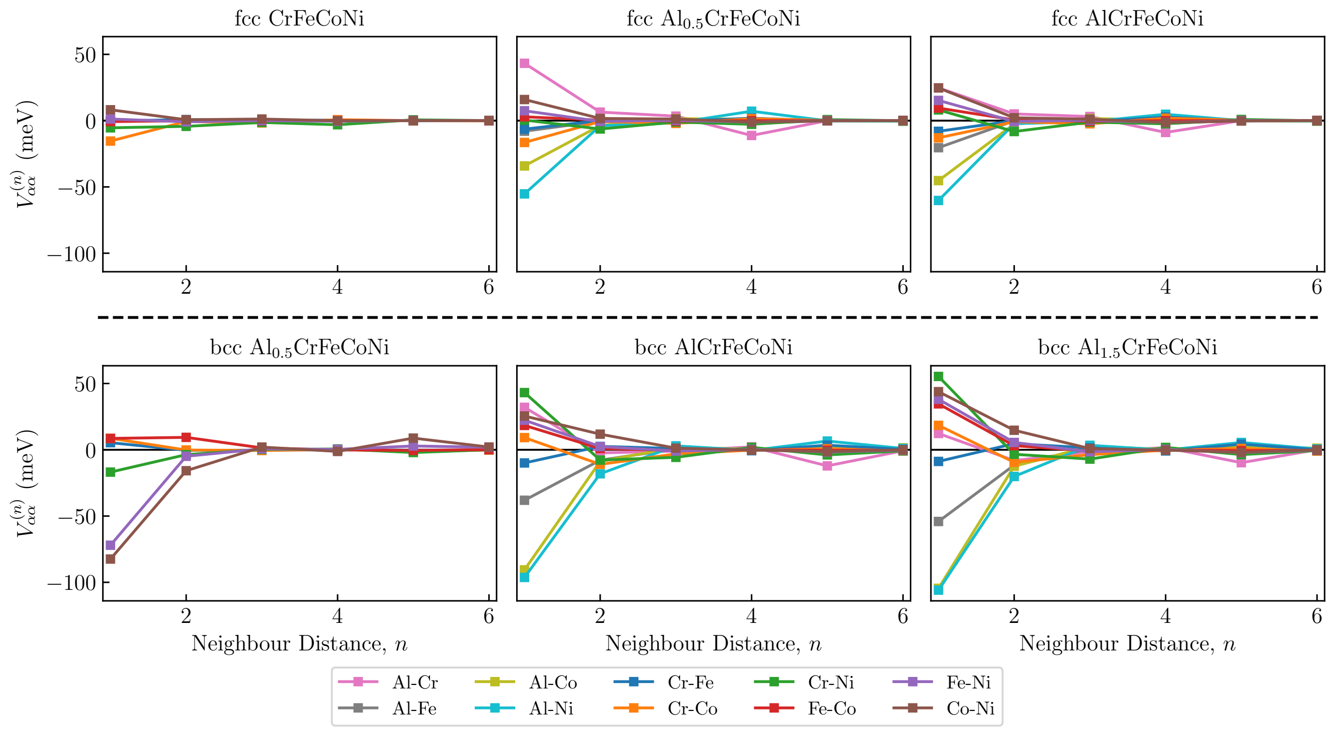


FIG. 4. Visualisation of the fitted effective pair interactions for unlike pairs for selected values of $x$ on both the fcc and bcc lattice as a function of coordination shell, $n$, fitted to the first six coordination shells. It can be seen that interactions are dominated by the nearest-neighbour interactions, and tail off quickly with increasing distance.

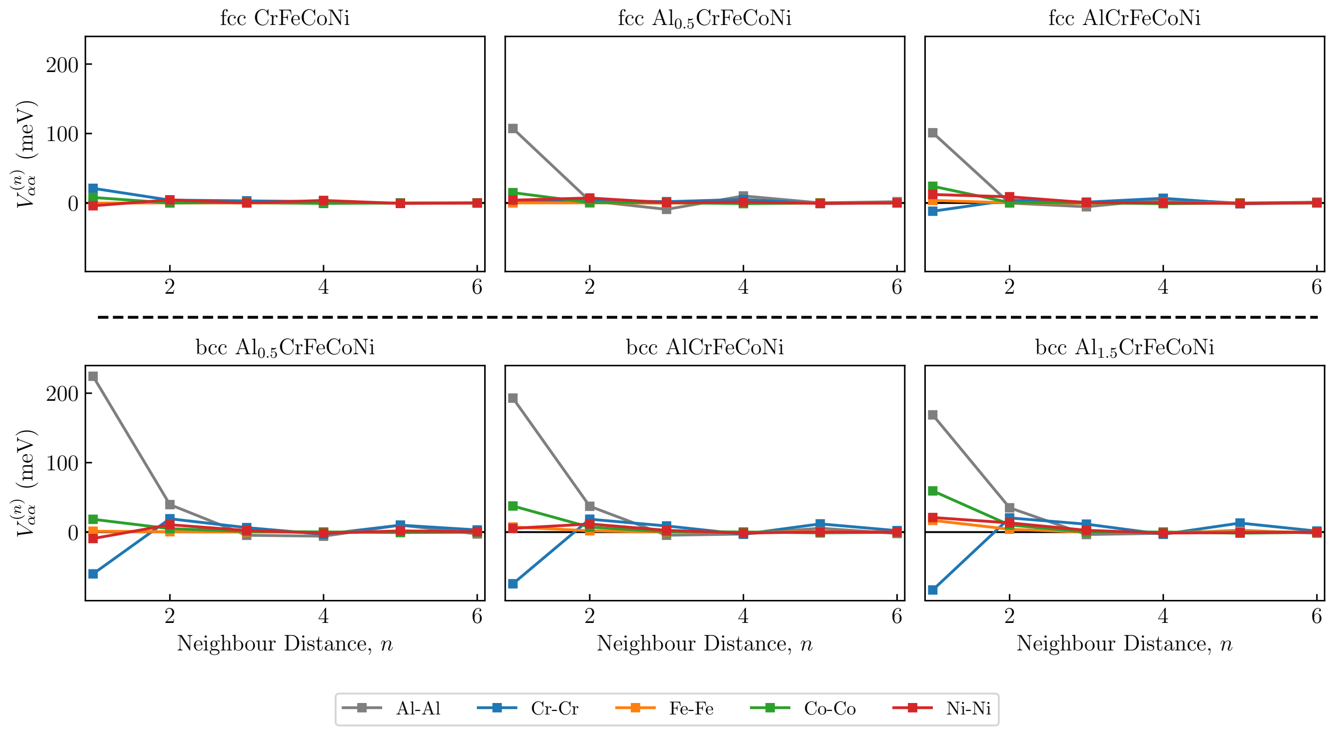


FIG. 5. Visualisation of the fitted effective pair interactions for like pairs for selected values of $x$ on both the fcc and bcc lattice as a function of coordination shell, $n$, fitted to the first six coordination shells. It can be seen that interactions are dominated by the nearest-neighbour interactions, and tail off quickly with increasing distance.

| $V^{(1)}_{\alpha\alpha'}$ | Ni | Co | Fe | Cr |
|---|---|---|---|---|
| Ni | −4.1 | 8.1 | 1.2 | −5.3 |
| Co | 8.1 | 7.9 | −0.7 | −15.3 |
| Fe | 1.2 | −0.7 | −0.3 | −0.3 |
| Cr | −5.3 | −15.3 | −0.3 | 20.9 |

| $V^{(2)}_{\alpha\alpha'}$ | Ni | Co | Fe | Cr |
|---|---|---|---|---|
| Ni | 4.7 | 0.8 | −0.9 | −4.6 |
| Co | 0.8 | 0.0 | −0.1 | −0.7 |
| Fe | −0.9 | −0.1 | 0.1 | 0.8 |
| Cr | −4.6 | −0.7 | 0.8 | 4.5 |

| $V^{(3)}_{\alpha\alpha'}$ | Ni | Co | Fe | Cr |
|---|---|---|---|---|
| Ni | 0.1 | 1.2 | 0.1 | −1.5 |
| Co | 1.2 | 0.6 | −0.1 | −1.7 |
| Fe | 0.1 | −0.1 | −0.0 | 0.1 |
| Cr | −1.5 | −1.7 | 0.1 | 3.1 |

| $V^{(4)}_{\alpha\alpha'}$ | Ni | Co | Fe | Cr |
|---|---|---|---|---|
| Ni | 3.8 | −0.0 | −0.5 | −3.3 |
| Co | −0.0 | −0.7 | −0.0 | 0.7 |
| Fe | −0.5 | −0.0 | 0.1 | 0.4 |
| Cr | −3.3 | 0.7 | 0.4 | 2.2 |

| $V^{(5)}_{\alpha\alpha'}$ | Ni | Co | Fe | Cr |
|---|---|---|---|---|
| Ni | −0.6 | −0.0 | 0.1 | 0.6 |
| Co | −0.0 | 0.1 | 0.0 | −0.0 |
| Fe | 0.1 | 0.0 | −0.0 | −0.1 |
| Cr | 0.6 | −0.0 | −0.1 | −0.4 |

| $V^{(6)}_{\alpha\alpha'}$ | Ni | Co | Fe | Cr |
|---|---|---|---|---|
| Ni | −0.2 | −0.0 | 0.0 | 0.2 |
| Co | −0.0 | 0.2 | 0.0 | −0.2 |
| Fe | 0.0 | 0.0 | −0.0 | −0.0 |
| Cr | 0.2 | −0.2 | −0.0 | −0.0 |

TABLE II. Fitted pairwise interactions on the fcc lattice for the CrFeCoNi alloy. (*I.e.*, $Al_x$CrFeCoNi, $x = 0$.) The interaction is fitted to the first six coordination shells of the fcc lattice. All energies in units of meV.

| $V^{(1)}_{\alpha\alpha'}$ | Al | Ni | Co | Fe | Cr |
|---|---|---|---|---|---|
| Al | 107.1 | −55.2 | −34.1 | −8.0 | 43.3 |
| Ni | −55.2 | 4.0 | 15.9 | 7.4 | 0.5 |
| Co | −34.1 | 15.9 | 14.9 | 2.9 | −16.4 |
| Fe | −8.0 | 7.4 | 2.9 | 0.1 | −6.4 |
| Cr | 43.3 | 0.5 | −16.4 | −6.4 | 0.5 |

| $V^{(2)}_{\alpha\alpha'}$ | Al | Ni | Co | Fe | Cr |
|---|---|---|---|---|---|
| Al | 3.0 | −3.8 | −3.6 | −0.4 | 6.3 |
| Ni | −3.8 | 7.3 | 1.7 | −0.6 | −6.5 |
| Co | −3.6 | 1.7 | 0.5 | 0.4 | −0.8 |
| Fe | −0.4 | −0.6 | 0.4 | 0.2 | 0.2 |
| Cr | 6.3 | −6.5 | −0.8 | 0.2 | 3.8 |

| $V^{(3)}_{\alpha\alpha'}$ | Al | Ni | Co | Fe | Cr |
|---|---|---|---|---|---|
| Al | −9.0 | −1.6 | 1.6 | 1.4 | 3.2 |
| Ni | −1.6 | 0.5 | 1.2 | 0.2 | −1.1 |
| Co | 1.6 | 1.2 | 0.4 | −0.3 | −2.0 |
| Fe | 1.4 | 0.2 | −0.3 | −0.2 | −0.4 |
| Cr | 3.2 | −1.1 | −2.0 | −0.4 | 2.0 |

| $V^{(4)}_{\alpha\alpha'}$ | Al | Ni | Co | Fe | Cr |
|---|---|---|---|---|---|
| Al | 10.1 | 7.2 | 1.3 | −2.2 | −11.4 |
| Ni | 7.2 | 1.5 | −1.1 | −1.2 | −2.9 |
| Co | 1.3 | −1.1 | −1.0 | −0.0 | 1.4 |
| Fe | −2.2 | −1.2 | −0.0 | 0.4 | 1.9 |
| Cr | −11.4 | −2.9 | 1.4 | 1.9 | 5.3 |

| $V^{(5)}_{\alpha\alpha'}$ | Al | Ni | Co | Fe | Cr |
|---|---|---|---|---|---|
| Al | 0.4 | −0.2 | −0.0 | 0.0 | 0.0 |
| Ni | −0.2 | −0.6 | −0.2 | 0.1 | 0.8 |
| Co | −0.0 | −0.2 | −0.1 | 0.0 | 0.2 |
| Fe | 0.0 | 0.1 | 0.0 | −0.0 | −0.1 |
| Cr | 0.0 | 0.8 | 0.2 | −0.1 | −0.9 |

| $V^{(6)}_{\alpha\alpha'}$ | Al | Ni | Co | Fe | Cr |
|---|---|---|---|---|---|
| Al | 2.1 | −0.4 | −0.6 | −0.2 | 0.2 |
| Ni | −0.4 | 0.0 | 0.0 | 0.0 | 0.1 |
| Co | −0.6 | 0.0 | 0.2 | 0.1 | −0.0 |
| Fe | −0.2 | 0.0 | 0.1 | 0.0 | −0.0 |
| Cr | 0.2 | 0.1 | −0.0 | −0.0 | −0.1 |

TABLE III. Fitted pairwise interactions for the $Al_{0.5}$CrFeCoNi alloy on the fcc lattice. (*I.e.*, $Al_x$CrFeCoNi, $x = 0.5$.) The interaction is fitted to the first six coordination shells of the fcc lattice. All energies in units of meV.

| $V^{(1)}_{\alpha\alpha'}$ | Al | Ni | Co | Fe | Cr |
|---|---|---|---|---|---|
| Al | 100.9 | −60.1 | −45.2 | −20.4 | 24.7 |
| Ni | −60.1 | 12.1 | 24.6 | 15.3 | 8.1 |
| Co | −45.2 | 24.6 | 24.0 | 9.5 | −12.9 |
| Fe | −20.4 | 15.3 | 9.5 | 3.7 | −8.0 |
| Cr | 24.7 | 8.1 | −12.9 | −8.0 | −11.9 |

| $V^{(2)}_{\alpha\alpha'}$ | Al | Ni | Co | Fe | Cr |
|---|---|---|---|---|---|
| Al | −0.2 | −2.3 | −2.5 | −0.1 | 5.1 |
| Ni | −2.3 | 9.1 | 2.2 | −0.6 | −8.3 |
| Co | −2.5 | 2.2 | 0.6 | 0.5 | −0.9 |
| Fe | −0.1 | −0.6 | 0.5 | 0.2 | −0.0 |
| Cr | 5.1 | −8.3 | −0.9 | −0.0 | 4.2 |

| $V^{(3)}_{\alpha\alpha'}$ | Al | Ni | Co | Fe | Cr |
|---|---|---|---|---|---|
| Al | −5.0 | −0.8 | 1.5 | 1.5 | 2.9 |
| Ni | −0.8 | 0.7 | 1.1 | 0.2 | −1.2 |
| Co | 1.5 | 1.1 | 0.2 | −0.5 | −2.3 |
| Fe | 1.5 | 0.2 | −0.5 | −0.4 | −0.7 |
| Cr | 2.9 | −1.2 | −2.3 | −0.7 | 1.4 |

| $V^{(4)}_{\alpha\alpha'}$ | Al | Ni | Co | Fe | Cr |
|---|---|---|---|---|---|
| Al | 5.5 | 4.8 | 0.7 | −2.0 | −9.0 |
| Ni | 4.8 | 0.5 | −1.4 | −1.4 | −2.5 |
| Co | 0.7 | −1.4 | −1.1 | −0.0 | 1.8 |
| Fe | −2.0 | −1.4 | −0.0 | 0.7 | 2.7 |
| Cr | −9.0 | −2.5 | 1.8 | 2.7 | 7.0 |

| $V^{(5)}_{\alpha\alpha'}$ | Al | Ni | Co | Fe | Cr |
|---|---|---|---|---|---|
| Al | 0.1 | −0.1 | −0.0 | 0.0 | −0.0 |
| Ni | −0.1 | −0.7 | −0.3 | 0.1 | 0.9 |
| Co | −0.0 | −0.3 | −0.1 | 0.0 | 0.4 |
| Fe | 0.0 | 0.1 | 0.0 | −0.0 | −0.1 |
| Cr | −0.0 | 0.9 | 0.4 | −0.1 | −1.2 |

| $V^{(6)}_{\alpha\alpha'}$ | Al | Ni | Co | Fe | Cr |
|---|---|---|---|---|---|
| Al | 1.2 | −0.3 | −0.5 | −0.3 | −0.1 |
| Ni | −0.3 | 0.2 | 0.1 | 0.1 | −0.0 |
| Co | −0.5 | 0.1 | 0.2 | 0.1 | 0.1 |
| Fe | −0.3 | 0.1 | 0.1 | 0.1 | 0.0 |
| Cr | −0.1 | −0.0 | 0.1 | 0.0 | 0.0 |

TABLE IV. Fitted pairwise interactions for the AlCrFeCoNi alloy on the fcc lattice. (*I.e.*, $Al_x$CrFeCoNi, $x = 1$.) The interaction is fitted to the first six coordination shells of the fcc lattice. All energies in units of meV.

| $V^{(1)}_{\alpha\alpha'}$ | Al | Ni | Co | Fe | Cr |
|---|---|---|---|---|---|
| Al | 95.3 | −65.4 | −55.3 | −31.3 | 9.7 |
| Ni | −65.4 | 21.0 | 34.8 | 24.7 | 17.3 |
| Co | −55.3 | 34.8 | 35.6 | 18.7 | −6.3 |
| Fe | −31.3 | 24.7 | 18.7 | 9.8 | −6.4 |
| Cr | 9.7 | 17.3 | −6.3 | −6.4 | −19.0 |

| $V^{(2)}_{\alpha\alpha'}$ | Al | Ni | Co | Fe | Cr |
|---|---|---|---|---|---|
| Al | −3.1 | −0.9 | −0.9 | 0.9 | 5.6 |
| Ni | −0.9 | 10.3 | 2.4 | −1.0 | −10.4 |
| Co | −0.9 | 2.4 | 0.3 | 0.3 | −1.6 |
| Fe | 0.9 | −1.0 | 0.3 | −0.0 | −0.5 |
| Cr | 5.6 | −10.4 | −1.6 | −0.5 | 4.2 |

| $V^{(3)}_{\alpha\alpha'}$ | Al | Ni | Co | Fe | Cr |
|---|---|---|---|---|---|
| Al | −2.7 | −0.4 | 1.2 | 1.2 | 2.1 |
| Ni | −0.4 | 0.8 | 1.0 | 0.2 | −1.4 |
| Co | 1.2 | 1.0 | 0.1 | −0.6 | −2.3 |
| Fe | 1.2 | 0.2 | −0.6 | −0.5 | −0.8 |
| Cr | 2.1 | −1.4 | −2.3 | −0.8 | 1.4 |

| $V^{(4)}_{\alpha\alpha'}$ | Al | Ni | Co | Fe | Cr |
|---|---|---|---|---|---|
| Al | 2.5 | 3.6 | 0.8 | −1.4 | −6.8 |
| Ni | 3.6 | −0.1 | −1.6 | −1.5 | −2.3 |
| Co | 0.8 | −1.6 | −1.3 | −0.2 | 1.8 |
| Fe | −1.4 | −1.5 | −0.2 | 0.7 | 3.0 |
| Cr | −6.8 | −2.3 | 1.8 | 3.0 | 7.6 |

| $V^{(5)}_{\alpha\alpha'}$ | Al | Ni | Co | Fe | Cr |
|---|---|---|---|---|---|
| Al | −0.2 | 0.1 | 0.0 | 0.1 | 0.1 |
| Ni | 0.1 | −0.7 | −0.4 | 0.0 | 1.0 |
| Co | 0.0 | −0.4 | −0.2 | 0.0 | 0.5 |
| Fe | 0.1 | 0.0 | 0.0 | −0.0 | −0.1 |
| Cr | 0.1 | 1.0 | 0.5 | −0.1 | −1.4 |

| $V^{(6)}_{\alpha\alpha'}$ | Al | Ni | Co | Fe | Cr |
|---|---|---|---|---|---|
| Al | 0.7 | −0.2 | −0.4 | −0.3 | −0.2 |
| Ni | −0.2 | 0.2 | 0.1 | 0.1 | −0.1 |
| Co | −0.4 | 0.1 | 0.2 | 0.1 | 0.1 |
| Fe | −0.3 | 0.1 | 0.1 | 0.1 | 0.1 |
| Cr | −0.2 | −0.1 | 0.1 | 0.1 | 0.2 |

TABLE V. Fitted pairwise interactions for the $Al_{1.5}$CrFeCoNi alloy on the fcc lattice. (*I.e.*, $Al_x$CrFeCoNi, $x = 1.5$.) The interaction is fitted to the first six coordination shells of the fcc lattice. All energies in units of meV.

| $V^{(1)}_{\alpha\alpha'}$ | Al | Ni | Co | Fe | Cr | $V^{(2)}_{\alpha\alpha'}$ | Al | Ni | Co | Fe | Cr |
|---|---|---|---|---|---|---|---|---|---|---|---|
| Al | 87.3 | −69.4 | −63.2 | −40.5 | −3.6 | Al | −5.4 | 0.7 | 0.9 | 2.3 | 7.0 |
| Ni | −69.4 | 30.3 | 45.9 | 35.7 | 28.5 | Ni | 0.7 | 11.2 | 2.3 | −1.8 | −13.0 |
| Co | −63.2 | 45.9 | 48.6 | 30.1 | 3.3 | Co | 0.9 | 2.3 | −0.5 | −0.5 | −3.1 |
| Fe | −40.5 | 35.7 | 30.1 | 18.2 | −2.1 | Fe | 2.3 | −1.8 | −0.5 | −0.7 | −1.6 |
| Cr | −3.6 | 28.5 | 3.3 | −2.1 | −22.4 | Cr | 7.0 | −13.0 | −3.1 | −1.6 | 3.5 |
| $V^{(3)}_{\alpha\alpha'}$ | Al | Ni | Co | Fe | Cr | $V^{(4)}_{\alpha\alpha'}$ | Al | Ni | Co | Fe | Cr |
| Al | −1.4 | −0.2 | 1.0 | 0.9 | 1.2 | Al | 0.6 | 3.0 | 1.1 | −0.7 | −4.7 |
| Ni | −0.2 | 0.9 | 0.9 | 0.1 | −1.6 | Ni | 3.0 | −0.4 | −1.7 | −1.7 | −2.2 |
| Co | 1.0 | 0.9 | 0.0 | −0.7 | −2.3 | Co | 1.1 | −1.7 | −1.5 | −0.4 | 1.4 |
| Fe | 0.9 | 0.1 | −0.7 | −0.6 | −0.7 | Fe | −0.7 | −1.7 | −0.4 | 0.6 | 2.9 |
| Cr | 1.2 | −1.6 | −2.3 | −0.7 | 2.1 | Cr | −4.7 | −2.2 | 1.4 | 2.9 | 7.5 |
| $V^{(5)}_{\alpha\alpha'}$ | Al | Ni | Co | Fe | Cr | $V^{(6)}_{\alpha\alpha'}$ | Al | Ni | Co | Fe | Cr |
| Al | −0.4 | 0.2 | 0.1 | 0.2 | 0.2 | Al | 0.4 | −0.1 | −0.2 | −0.2 | −0.2 |
| Ni | 0.2 | −0.8 | −0.5 | −0.0 | 0.9 | Ni | −0.1 | 0.3 | 0.1 | 0.0 | −0.2 |
| Co | 0.1 | −0.5 | −0.3 | −0.0 | 0.5 | Co | −0.2 | 0.1 | 0.2 | 0.1 | 0.1 |
| Fe | 0.2 | −0.0 | −0.0 | −0.1 | −0.2 | Fe | −0.2 | 0.0 | 0.1 | 0.1 | 0.1 |
| Cr | 0.2 | 0.9 | 0.5 | −0.2 | −1.7 | Cr | −0.2 | −0.2 | 0.1 | 0.1 | 0.4 |

TABLE VI. Fitted pairwise interactions for the $Al_2CrFeCoNi$ alloy on the fcc lattice. (*I.e.*, $Al_x$CrFeCoNi, $x = 2$.) The interaction is fitted to the first six coordination shells of the fcc lattice. All energies in units of meV.

| $V^{(1)}_{\alpha\alpha'}$ | Ni | Co | Fe | Cr | $V^{(2)}_{\alpha\alpha'}$ | Ni | Co | Fe | Cr |
|---|---|---|---|---|---|---|---|---|---|
| Ni | −20.3 | −5.1 | −1.4 | 26.8 | Ni | 9.0 | 7.0 | −2.2 | −13.8 |
| Co | −5.1 | 3.5 | −2.7 | 4.4 | Co | 7.0 | 3.7 | −0.8 | −9.9 |
| Fe | −1.4 | −2.7 | 0.8 | 3.3 | Fe | −2.2 | −0.8 | 0.3 | 2.8 |
| Cr | 26.8 | 4.4 | 3.3 | −34.5 | Cr | −13.8 | −9.9 | 2.8 | 20.9 |
| $V^{(3)}_{\alpha\alpha'}$ | Ni | Co | Fe | Cr | $V^{(4)}_{\alpha\alpha'}$ | Ni | Co | Fe | Cr |
| Ni | 1.8 | 1.2 | −0.3 | −2.8 | Ni | −1.4 | −0.1 | −0.1 | 1.6 |
| Co | 1.2 | 0.9 | −0.2 | −1.8 | Co | −0.1 | 0.2 | −0.1 | −0.1 |
| Fe | −0.3 | −0.2 | 0.1 | 0.4 | Fe | −0.1 | −0.1 | 0.0 | 0.1 |
| Cr | −2.8 | −1.8 | 0.4 | 4.2 | Cr | 1.6 | −0.1 | 0.1 | −1.6 |
| $V^{(5)}_{\alpha\alpha'}$ | Ni | Co | Fe | Cr | $V^{(6)}_{\alpha\alpha'}$ | Ni | Co | Fe | Cr |
| Ni | 3.8 | 0.9 | 0.1 | −4.8 | Ni | 0.6 | 0.2 | 0.1 | −0.9 |
| Co | 0.9 | 0.1 | 0.1 | −1.1 | Co | 0.2 | 0.1 | 0.0 | −0.4 |
| Fe | 0.1 | 0.1 | −0.1 | −0.1 | Fe | 0.1 | 0.0 | −0.0 | −0.1 |
| Cr | −4.8 | −1.1 | −0.1 | 5.9 | Cr | −0.9 | −0.4 | −0.1 | 1.3 |

TABLE VII. Fitted pairwise interactions on the bcc lattice for the CrFeCoNi alloy. (*I.e.*, $Al_x$CrFeCoNi, $x = 0$.) The interaction is fitted to the first six coordination shells of the bcc lattice. All energies in units of meV.

| $V^{(1)}_{\alpha\alpha'}$ | Al | Ni | Co | Fe | Cr | $V^{(2)}_{\alpha\alpha'}$ | Al | Ni | Co | Fe | Cr |
|---|---|---|---|---|---|---|---|---|---|---|---|
| Al | 223.3 | −82.9 | −72.0 | −16.7 | 59.0 | Al | 40.7 | −15.1 | −4.7 | −3.9 | 3.2 |
| Ni | −82.9 | −9.7 | 8.4 | 8.7 | 34.4 | Ni | −15.1 | 11.5 | 9.7 | −0.3 | −13.2 |
| Co | −72.0 | 8.4 | 18.4 | 5.4 | 4.2 | Co | −4.7 | 9.7 | 5.1 | −0.5 | −11.9 |
| Fe | −16.7 | 8.7 | 5.4 | 1.3 | −6.9 | Fe | −3.9 | −0.3 | −0.5 | 0.6 | 2.1 |
| Cr | 59.0 | 34.4 | 4.2 | −6.9 | −61.3 | Cr | 3.2 | −13.2 | −11.9 | 2.1 | 21.4 |
| $V^{(3)}_{\alpha\alpha'}$ | Al | Ni | Co | Fe | Cr | $V^{(4)}_{\alpha\alpha'}$ | Al | Ni | Co | Fe | Cr |
| Al | −4.0 | 3.8 | 1.6 | 0.0 | −3.3 | Al | −6.2 | −2.1 | −0.0 | 0.7 | 4.5 |
| Ni | 3.8 | 3.6 | 1.7 | −0.8 | −6.5 | Ni | −2.1 | −2.3 | −0.4 | 0.4 | 3.3 |
| Co | 1.6 | 1.7 | 1.0 | −0.4 | −3.2 | Co | −0.0 | −0.4 | 0.1 | −0.0 | 0.2 |
| Fe | 0.0 | −0.8 | −0.4 | 0.1 | 1.1 | Fe | 0.7 | 0.4 | −0.0 | −0.1 | −0.7 |
| Cr | −3.3 | −6.5 | −3.2 | 1.1 | 10.2 | Cr | 4.5 | 3.3 | 0.2 | −0.7 | −5.2 |
| $V^{(5)}_{\alpha\alpha'}$ | Al | Ni | Co | Fe | Cr | $V^{(6)}_{\alpha\alpha'}$ | Al | Ni | Co | Fe | Cr |
| Al | 10.7 | 9.7 | 3.2 | −2.2 | −16.1 | Al | −2.5 | 2.1 | 1.9 | 0.0 | −2.8 |
| Ni | 9.7 | 2.5 | −0.3 | −1.3 | −5.9 | Ni | 2.1 | 0.6 | 0.1 | −0.2 | −1.5 |
| Co | 3.2 | −0.3 | −0.6 | −0.3 | −0.4 | Co | 1.9 | 0.1 | −0.2 | −0.2 | −0.7 |
| Fe | −2.2 | −1.3 | −0.3 | 0.4 | 2.3 | Fe | 0.0 | −0.2 | −0.2 | 0.0 | 0.4 |
| Cr | −16.1 | −5.9 | −0.4 | 2.3 | 12.1 | Cr | −2.8 | −1.5 | −0.7 | 0.4 | 3.2 |

TABLE VIII. Fitted pairwise interactions for the $Al_{0.5}CrFeCoNi$ alloy on the bcc lattice. (*I.e.*, $Al_x$CrFeCoNi, $x = 0.5$.) The interaction is fitted to the first six coordination shells of the bcc lattice. All energies in units of meV.

| $V^{(1)}_{\alpha\alpha'}$ | Al | Ni | Co | Fe | Cr | $V^{(2)}_{\alpha\alpha'}$ | Al | Ni | Co | Fe | Cr |
|---|---|---|---|---|---|---|---|---|---|---|---|
| Al | 192.6 | −96.5 | −90.5 | −38.0 | 32.4 | Al | 37.7 | −17.9 | −8.8 | −8.0 | −2.9 |
| Ni | −96.5 | 5.1 | 25.3 | 22.4 | 43.6 | Ni | −17.9 | 12.2 | 12.0 | 2.4 | −8.6 |
| Co | −90.5 | 25.3 | 37.5 | 18.4 | 9.3 | Co | −8.8 | 12.0 | 7.2 | 0.9 | −11.3 |
| Fe | −38.0 | 22.4 | 18.4 | 7.3 | −10.1 | Fe | −8.0 | 2.4 | 0.9 | 2.0 | 2.8 |
| Cr | 32.4 | 43.6 | 9.3 | −10.1 | −75.3 | Cr | −2.9 | −8.6 | −11.3 | 2.8 | 20.0 |
| $V^{(3)}_{\alpha\alpha'}$ | Al | Ni | Co | Fe | Cr | $V^{(4)}_{\alpha\alpha'}$ | Al | Ni | Co | Fe | Cr |
| Al | −4.3 | 3.6 | 2.3 | 0.5 | −2.1 | Al | −2.6 | −0.8 | 0.2 | 0.7 | 2.6 |
| Ni | 3.6 | 3.2 | 1.4 | −1.2 | −7.0 | Ni | −0.8 | −1.8 | −0.3 | 0.4 | 2.6 |
| Co | 2.3 | 1.4 | 0.6 | −0.7 | −3.5 | Co | 0.2 | −0.3 | 0.2 | −0.0 | 0.0 |
| Fe | 0.5 | −1.2 | −0.7 | 0.0 | 1.4 | Fe | 0.7 | 0.4 | −0.0 | −0.2 | −0.9 |
| Cr | −2.1 | −7.0 | −3.5 | 1.4 | 11.3 | Cr | 2.6 | 2.6 | 0.0 | −0.9 | −4.3 |
| $V^{(5)}_{\alpha\alpha'}$ | Al | Ni | Co | Fe | Cr | $V^{(6)}_{\alpha\alpha'}$ | Al | Ni | Co | Fe | Cr |
| Al | 5.8 | 6.9 | 2.3 | −2.2 | −12.8 | Al | −1.9 | 1.0 | 1.5 | 0.3 | −0.9 |
| Ni | 6.9 | 0.7 | −1.2 | −1.8 | −4.6 | Ni | 1.0 | 0.1 | −0.0 | −0.2 | −0.8 |
| Co | 2.3 | −1.2 | −1.1 | −0.4 | 0.5 | Co | 1.5 | −0.0 | −0.3 | −0.3 | −0.8 |
| Fe | −2.2 | −1.8 | −0.4 | 0.7 | 3.7 | Fe | 0.3 | −0.2 | −0.3 | −0.0 | 0.3 |
| Cr | −12.8 | −4.6 | 0.5 | 3.7 | 13.2 | Cr | −0.9 | −0.8 | −0.8 | 0.3 | 2.2 |

TABLE IX. Fitted pairwise interactions for the AlCrFeCoNi alloy on the bcc lattice. (*I.e.*, $Al_x$CrFeCoNi, $x = 1$.) The interaction is fitted to the first six coordination shells of the bcc lattice. All energies in units of meV.

| $V^{(1)}_{\alpha\alpha'}$ | Al | Ni | Co | Fe | Cr | $V^{(2)}_{\alpha\alpha'}$ | Al | Ni | Co | Fe | Cr |
|---|---|---|---|---|---|---|---|---|---|---|---|
| Al | 168.7 | −106.0 | −104.5 | −54.1 | 12.5 | Al | 35.4 | −20.1 | −12.5 | −11.8 | −8.6 |
| Ni | −106.0 | 20.8 | 43.7 | 38.2 | 55.7 | Ni | −20.1 | 13.6 | 14.9 | 5.5 | −4.0 |
| Co | −104.5 | 43.7 | 59.3 | 34.7 | 18.6 | Co | −12.5 | 14.9 | 10.4 | 3.1 | −9.7 |
| Fe | −54.1 | 38.2 | 34.7 | 16.9 | −8.9 | Fe | −11.8 | 5.5 | 3.1 | 4.2 | 4.8 |
| Cr | 12.5 | 55.7 | 18.6 | −8.9 | −84.1 | Cr | −8.6 | −4.0 | −9.7 | 4.8 | 21.7 |

| $V^{(3)}_{\alpha\alpha'}$ | Al | Ni | Co | Fe | Cr | $V^{(4)}_{\alpha\alpha'}$ | Al | Ni | Co | Fe | Cr |
|---|---|---|---|---|---|---|---|---|---|---|---|
| Al | −3.3 | 3.7 | 2.7 | 0.6 | −2.2 | Al | −1.4 | −0.5 | 0.2 | 0.6 | 1.8 |
| Ni | 3.7 | 3.1 | 1.0 | −1.7 | −8.0 | Ni | −0.5 | −1.7 | −0.3 | 0.4 | 2.4 |
| Co | 2.7 | 1.0 | 0.0 | −1.1 | −4.0 | Co | 0.2 | −0.3 | 0.2 | −0.0 | −0.0 |
| Fe | 0.6 | −1.7 | −1.1 | 0.0 | 1.8 | Fe | 0.6 | 0.4 | −0.0 | −0.3 | −1.0 |
| Cr | −2.2 | −8.0 | −4.0 | 1.8 | 13.4 | Cr | 1.8 | 2.4 | −0.0 | −1.0 | −4.0 |

| $V^{(5)}_{\alpha\alpha'}$ | Al | Ni | Co | Fe | Cr | $V^{(6)}_{\alpha\alpha'}$ | Al | Ni | Co | Fe | Cr |
|---|---|---|---|---|---|---|---|---|---|---|---|
| Al | 2.7 | 5.7 | 2.1 | −1.7 | −10.2 | Al | −1.5 | 0.6 | 1.2 | 0.5 | −0.1 |
| Ni | 5.7 | −0.2 | −1.8 | −2.2 | −4.2 | Ni | 0.6 | −0.0 | −0.0 | −0.2 | −0.6 |
| Co | 2.1 | −1.8 | −1.5 | −0.7 | 0.8 | Co | 1.2 | −0.0 | −0.3 | −0.4 | −1.0 |
| Fe | −1.7 | −2.2 | −0.7 | 0.9 | 4.5 | Fe | 0.5 | −0.2 | −0.4 | −0.1 | 0.1 |
| Cr | −10.2 | −4.2 | 0.8 | 4.5 | 14.2 | Cr | −0.1 | −0.6 | −1.0 | 0.1 | 1.6 |

TABLE X. Fitted pairwise interactions for the $Al_{1.5}CrFeCoNi$ alloy on the bcc lattice. (*I.e.*, $Al_xCrFeCoNi$, $x = 1.5$.) The interaction is fitted to the first six coordination shells of the bcc lattice. All energies in units of meV.

| $V^{(1)}_{\alpha\alpha'}$ | Al | Ni | Co | Fe | Cr | $V^{(2)}_{\alpha\alpha'}$ | Al | Ni | Co | Fe | Cr |
|---|---|---|---|---|---|---|---|---|---|---|---|
| Al | 149.1 | −113.0 | −116.3 | −67.7 | −4.9 | Al | 32.9 | −21.9 | −15.9 | −15.2 | −13.7 |
| Ni | −113.0 | 37.6 | 64.1 | 56.3 | 70.6 | Ni | −21.9 | 15.5 | 18.5 | 9.1 | 1.1 |
| Co | −116.3 | 64.1 | 84.5 | 54.7 | 32.0 | Co | −15.9 | 18.5 | 14.6 | 6.2 | −7.0 |
| Fe | −67.7 | 56.3 | 54.7 | 30.1 | −4.0 | Fe | −15.2 | 9.1 | 6.2 | 7.2 | 8.1 |
| Cr | −4.9 | 70.6 | 32.0 | −4.0 | −88.8 | Cr | −13.7 | 1.1 | −7.0 | 8.1 | 25.6 |

| $V^{(3)}_{\alpha\alpha'}$ | Al | Ni | Co | Fe | Cr | $V^{(4)}_{\alpha\alpha'}$ | Al | Ni | Co | Fe | Cr |
|---|---|---|---|---|---|---|---|---|---|---|---|
| Al | −1.9 | 3.6 | 2.7 | 0.4 | −2.8 | Al | −0.9 | −0.3 | 0.2 | 0.6 | 1.4 |
| Ni | 3.6 | 3.1 | 0.7 | −2.2 | −8.9 | Ni | −0.3 | −1.7 | −0.4 | 0.4 | 2.3 |
| Co | 2.7 | 0.7 | −0.5 | −1.4 | −4.3 | Co | 0.2 | −0.4 | 0.2 | −0.1 | −0.1 |
| Fe | 0.4 | −2.2 | −1.4 | 0.1 | 2.6 | Fe | 0.6 | 0.4 | −0.1 | −0.4 | −1.2 |
| Cr | −2.8 | −8.9 | −4.3 | 2.6 | 16.3 | Cr | 1.4 | 2.3 | −0.1 | −1.2 | −4.0 |

| $V^{(5)}_{\alpha\alpha'}$ | Al | Ni | Co | Fe | Cr | $V^{(6)}_{\alpha\alpha'}$ | Al | Ni | Co | Fe | Cr |
|---|---|---|---|---|---|---|---|---|---|---|---|
| Al | 0.6 | 5.0 | 2.4 | −0.8 | −7.8 | Al | −1.0 | 0.4 | 0.9 | 0.5 | 0.3 |
| Ni | 5.0 | −1.0 | −2.4 | −2.7 | −4.2 | Ni | 0.4 | −0.1 | −0.0 | −0.2 | −0.5 |
| Co | 2.4 | −2.4 | −2.1 | −1.1 | 0.6 | Co | 0.9 | −0.0 | −0.3 | −0.5 | −1.1 |
| Fe | −0.8 | −2.7 | −1.1 | 0.7 | 4.7 | Fe | 0.5 | −0.2 | −0.5 | −0.2 | −0.1 |
| Cr | −7.8 | −4.2 | 0.6 | 4.7 | 14.6 | Cr | 0.3 | −0.5 | −1.1 | −0.1 | 1.1 |

TABLE XI. Fitted pairwise interactions for the $Al_2CrFeCoNi$ alloy on the bcc lattice. (*I.e.*, $Al_xCrFeCoNi$, $x = 2$.) The interaction is fitted to the first six coordination shells of the bcc lattice. All energies in units of meV.
